# Supplementary material for: Physics-Informed Graph Neural Network Surrogates for Turbulent Nanoparticle Dispersion in Dental Clinical Environments
Source: arXiv:2605.19589 source file (2026-05-19)
Supplement: Supplementary file 1 [file paper_si_xref_stubs.tex]

\makeatletter
\def\si@maybe@set@ref#1#2{%
  \expandafter\ifx\csname r@#1\endcsname\relax
    \expandafter\def\csname r@#1\endcsname{{#2}{1}}%
  \fi
}

\si@maybe@set@ref{sec:training}{IV}
\si@maybe@set@ref{sec:results}{V}
\si@maybe@set@ref{tab:results}{III}
\si@maybe@set@ref{eq:euler_node_feat}{8}
\si@maybe@set@ref{eq:lag_node_feat}{10}
\si@maybe@set@ref{eq:idw}{12}
\makeatother
